# Supplementary material for: When soft crystals defy Newton's third law: Non-reciprocal mechanics and dislocation motility
Source: arXiv:2110.02897 source file (2021-10-07)

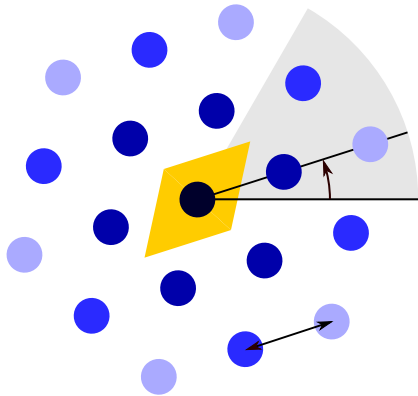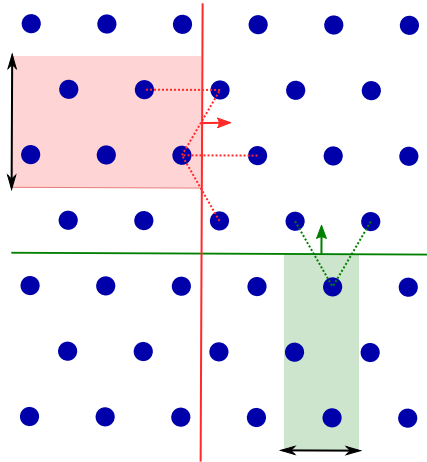

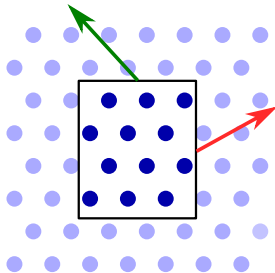

Supplement: Supplementary file 1 [file fig_sm2.pdf]
